# Supplementary material for: Malicious Network Traffic Detection via Deep Learning: An Information Theoretic View
Source: arXiv:2009.07753 source file (2020-09-16)
Supplement: Supplementary file 1 [file 14-appendix-2.tex]

\footnotesize
% Setup and stylize appendices to integrate with TOC
\addtocontents{toc}{\protect\renewcommand\protect\cftchappresnum{\appendixname~}}

% Stylize section header

%\addcontentsline{toc}{chapter}{Oligonucleotide and probe sequences}
\chapter{Mutual Information Estimation}
\label{append:two}

Our entropy estimation\footnote{Code is available at https://github.com/erickgalinkin/jhu\_masters/tree/master/code} relies on calculating the unique probabilities of values in our dataset and labels, as well as methods from Schwartz-Ziv and Tishby~\cite{shwartz2017opening} to compute the information using bins. 

\section{Methodology}
First, we compute the probabilities of the labels, and assign those values to a variable.
